# Supplementary material for: Experimental evidence of accelerated seismic release without critical failure in acoustic emissions of compressed nanoporous materials
Source: arXiv:1803.09293 ancillary file (2018-03-25)
Supplement: Supplementary file 1 [file ExperimentalEvidencesBaroetal2018_Sup.pdf]

# Experimental evidence of accelerated seismic release without critical failure in acoustic emissions of compressed nanoporous materials: Supplementary Material.

Jordi Baró,[1, 2, 3, *] Karin A. Dahmen,[1] Jörn Davidsen,[2] Antoni Planes,[3] Pedro O. Castillo,[3, 4] Guillaume F. Nataf,[3, 5] Ekhard K. H. Salje,[6] and Eduard Vives[3, †]

[1]*Department of Physics, University of Illinois at Urbana Champaign,Urbana, Illinois 61801, USA.*

[2]*Department of Physics and Astronomy University of Calgary. 2500 University Drive NW Calgary, Alberta T2N 1N4, Canada.*

[3]*Departament de Física de la Matèria Condensada. Facultat de Física. Universitat de Barcelona. Martí i Franquès, 1. 08028 Barcelona, Catalonia.*

[4]*CONACYT, Instituto Tecnológico de Oaxaca, Av. Ing. Víctor Bravo Ahuja 125, Oaxaca de Juárez 68030, México.*

[5]*Department of Materials Science, University of Cambridge, 27 Charles Babbage Road, Cambridge CB3 0FS, UK.*

[6]*Department of Earth Sciences, University of Cambridge, Downing Street, Cambridge CB2 3EQ, UK.*

The following is a comprehensive list of supplementary details supporting the manuscript *'Experimental evidence of accelerated seismic release without critical failure in acoustic emissions of compressed nanoporous materials'*, from now on referred to as Ref. [S1]. The content has been sorted to provide a straightforward reading. In Ref. [S1], the content is mentioned in a different order. The supplementary material is addressed for the first time in Ref. [S1] for the relation between the acoustic emission (AE) event magnitudes, here described in *Section III. Interpretation of the acoustic signals*. *Section IV. Distribution of AE energies* provides additional figures supporting the results summarized in Fig. 3 of Ref. [S1]. The formulation and differences between the two mean field (MF) models used as benchmarks is presented in *Section II. Mean field models of friction and fracture* and references therein. Finally, the theoretical relations between the energy exponents and the fundamental MF exponents are well established and summarized in *Section I. Exponent relations in the mean field theory.*

## I. Exponent relations in the mean field theory

The scaling relations and avalanche statistics in mean field (MF) theory are usually expressed in terms of avalanche sizes ($S$) measured as the sum of all individual events involved in the avalanche, such as slips in the slip mean field theory (SMFT) or broken fibers in DFB model. In micromechanical models, considering a linear relationship with the strain released ($S \propto \Delta\epsilon$) the size ($S$) is usually assumed to be proportional to the work of the external forces during the avalanche that will partly radiate as acoustic emission (AE) energy: $E_{AE}$. The presence of the dissipative processes, such as the ones associated to transient hardening, can introduce creep, reducing the fraction of energy that is released in sudden avalanches. As discussed in Ref. [S2], we assume that the amount of energy dissipated by creep can be linearized in a proportionality term, modifying the statistical properties only by a scalar factor. A summary of the relations between exponents can be found in Ref. [S3]. Here, we are interested in a list of exponents that can be derived from two fundamental scaling relations of the MF theory:

*Scaling of avalanche profiles*: According to the MF theory used here [S4], in the continuum limit, a temporal profile ($v(t)$) of slip velocities during an avalanche, as a function of time $t$ and averaged over all avalanches of the same duration $T$, is predicted to scale with $T$ as:

$$\langle v(t)|T\rangle = T^{\frac{1}{\sigma\nu z}-1}\tilde{v}(t/T), \tag{S1}$$

where $\tilde{v}(x)$ is a universal scaling function and the time origin has been set at the onset of the avalanche. The size of the avalanche is the time integral over the slip velocity time profile. The average size for avalanches during T scales in mean field theory as: $S = \int_{t=0}^{T} v(t)dt$, and, on average:

$$\langle S|T\rangle \propto T^{\frac{1}{\sigma\nu z}}. \tag{S2}$$

Considering that in mechanical avalanches the size is proportional to the seismic moment, $v(t)$ is proportional to the slip velocity, and the total kinetic energy ($E$) of the avalanche can be computed from the time integral over the slip velocity squared: $E = \int_{t=0}^{T} |v(t)|^2 dt$. Given the validity of Eq. (S1), on average this leads to the scaling form:

$$\langle E|T\rangle \propto T^{\frac{2}{\sigma\nu z}-1}. \tag{S3}$$

If the AE energy ($E_{AE}$) is proportional to the avalanche kinetic energy $E$, this relation establishes an equivalence between the MF theory and the exponent defined in the manuscript: $\gamma \equiv \frac{2}{\sigma\nu z} - 1$.

*Scaling close to criticality*: Exponents $\kappa$ and $\sigma$ are defined from the distribution of avalanche sizes. Close to criticality, the distribution of avalanche sizes is a generalized homogeneous function:

$$D(S;f)dS = S^{-\kappa}\mathcal{D}_S(Sf^{1/\sigma})dS = f^{\kappa/\sigma}\tilde{\mathcal{D}}_S(Sf^{1/\sigma}) \tag{S4}$$

similar to Eq. (2) in Ref. [S1], where $f := \sigma_c - \sigma$ is the distance to the critical point given in terms of stress ($\sigma$). The distribution of $E$ can be expressed in terms of these exponents as [S5]:

$$D(E;f)dE = E^{\frac{1-\kappa}{2-\sigma\nu z}-1}\mathcal{D}_E(Ef^{\frac{2-\sigma\nu z}{\sigma}})dE. \quad (S5)$$

Thus, the exponents used in the manuscript can be expressed in function of the previous ones as: $\varepsilon \equiv \frac{\kappa-1}{2-\sigma\nu z}+1$ and $\beta = \frac{2-\sigma\nu z}{\sigma}$, regardless of the driving mechanism. The exponents represented in Table II of Ref. [S1] are found from:

$$\begin{cases} \sigma\nu z \equiv \frac{2}{\gamma+1} \\ \kappa \equiv (2-\sigma\nu z)(\varepsilon-1)+1 \\ \sigma \equiv \frac{2-\sigma\nu z}{\beta} \end{cases} \quad (S6)$$

Finally, the relation between accelerated seismic release (ASR) and the above exponents is not clear and can have two different interpretations, as discussed in the body of the manuscript.

## II. Mean field models of friction and fracture

In the main text of this manuscript [S1], we compare the exponents estimated from the experiments with the mean field (MF) universality classes (UC) of friction and fracture avalanche processes, which differ in some aspects.

*Friction*: Starting from the Ben-Zion Rice (BZR) earthquake model [S6] we use both a discrete version and a continuum version of the corresponding mean field model developed in Refs. [S4, S7] (henceforth called the slip mean field model (SMFT) [S4]) as a benchmark for friction avalanches. A renormalization group approach was used in [S7] to show that the long range elastic interaction along the surface of an elastic half space are so long range that mean field theory gives the correct scaling behavior for the statistics and the dynamics of the slips on the frictional surface. In the mean field theory the long range elastic interactions are replaced with infinite range interactions, and the resulting model can be solved analytically [S4, S7]. The simple mean field model can be used to describe the micromechanical origin of seismic events as slip avalanches in a plastic shear flow regime and to gain the necessary intuition and guidance for the analysis of observational data. Even though the discrete version of the model at first looks somewhat similar to spring-blocks models [S8, S9], it differs from these models in several important ways: (1) It can be solved analytically, (2) it takes into account the long range character of the elastic interactions along a slip plane, (3) it does not concentrate the mass on the slipping surface but takes into account that the mass spread throughout the bulk, and it can be rewritten in an analytically solvable continuum version [S7]. During recent years, modified versions of the mean field model have been developed and solved as paradigms of slips inside solid materials for different loading conditions [S10–S12]. For example, the effects of tuning experimental parameters such as stress, strain-rate, and packing fraction in granular materials have been predicted in [S4, S13, S14]. The model predictions agree well with experiments and observations on amorphous, granular and crystalline matter, rocks, and earthquakes [S11, S12, S15–S19]. The basic idea of the model is that each cell $l$ is stuck until its stress surpasses a local failure stress $\tau_{f,l}$ which is chosen from a narrow random distribution. The exact shape of the distribution can be shown to be irrelevant for the statistical properties. Once a cell has slipped (by a random amount), a fraction of the released stress (which depends on the packing fraction or the a loading spring stiffness) is released to the other cells in the system. As a result additional cells can be triggered to slip as well, causing a slip avalanche of size $S$ proportional to the number of slips involved in the avalanche. The constitutive equation of the resulting shear flow, relating the evolution of stress ($\sigma(t)$) and a strain ($\epsilon(t)$) can be expressed as: $\sigma(t) = K(\epsilon(t) - \langle u\rangle(t))$, where $\langle u\rangle(t)$ is the mean displacement of the individual elements and $K$ an elastic modulus. A comprehensive list of the resulting MF exponents can be found in Ref. [S3, S5, S20].

*Fracture*: As a benchmark for fracture models, we use the democratic fiber bundle (DFB) model [S21], first used to describe the mechanical failure of non-braid bundles of fibers under tension, but later adapted to other mechanical fracture processes under different loadings [S22], even compression [S23]. In this case, each element $l$ breaks upon stretching a global strain ($\epsilon$) above a certain fixed strength value $s_{f,l}$. Once broken, the element disappears, creating an effective weakening of the system. In this case the constitutive equation can be expressed as: $\sigma = K\epsilon(1 - F(K\epsilon))$ where $F(K\epsilon)$ is the the fraction of broken fibers at $K\epsilon$ determined by the original strength of the fibers. Avalanches are defined from the dynamics of the broken fibers: the avalanche size $S$ is defined as the number of fibers broken within a single avalanche event. It is proportional to the increase in $F(K\epsilon)$. The critical power law exponents associated with the avalanche statistics discussed in this work are analytically obtained in Ref. [S2].

The most remarkable difference between the two MF models is the existence of an ultimate failure point in the DFB model and a critical flow regime under strain ($\epsilon$) driving in the SMFT. Since in both models $dS/dt \propto d\epsilon/df$, we use the approach to failure ($dS/dt(f)$) as

the lowest order expansion of the constitutive equation around the critical stress ($\sigma_c$). The strain rate depends on the distance $f$ to $\sigma_c$ as: $d\epsilon/dt \sim f^{(\kappa-2)/\sigma}$. Thus, in the stick-slip model, for which $(\kappa-2)/\sigma = -1$, the constitutive equation around $\sigma_c$ has a logarithmic approach to failure:

$$\epsilon(\sigma \to \sigma_c^-) \sim -\ln(1-\sigma/\sigma_c). \quad \text{(S7)}$$

Under strain driving, the stress $\sigma$ is asymptotically approached to the critical value, reaching an stationary flow regime with properties of self organized criticality. At the micromechanical level, this is possible because all the elements that slip, giving rise to $d\epsilon/dt$, are reintroduced to the system giving an extended tolerance to deformation in a recursive process. On the contrary, for the fiber bundle model, the amount of deformation with mechanical stability is limited, since each fiber is removed of the system once broken. Thus, the stable solution for strain cannot grow beyond a certain value, or failure point $\epsilon_c$, that is asymptotically critical in the standard MF model [S2]. Since $(\kappa-2)/\sigma = -0.5$ the expansion of $\epsilon$ around $\sigma_c$ reads:

$$\epsilon(\sigma \to \sigma_c^-) \sim 1-(1-\sigma/\sigma_c)^{1/2}, \quad \text{(S8)}$$

and has a solution at $\sigma_c$ for a finite strain value. Instead of the flow regime, a singular critical point is reach at failure.

### III. Interpretation of the acoustic signals

The interpretation of the measured AE energy in terms of the original internal avalanche is still a matter of debate and may depend on mechanism used by the AE sensors in the experiments. Let's consider that the elastic energy released during an avalanche is a consequence of a slip of a limited area $A$ with a temporal velocity profile $v(t)$. The profile $v(t)$ rises from initial zero velocity ($v(t=t_i)=0$) and finally drops again to zero velocity ($v(t=t_i+T)=0$) after a time $T$. The time $T$ is the duration of the avalanche. The 'velocity' of the avalanche is defined to be proportional to the seismic moment released per time unit: $v(t) \sim dM(t)$. A fraction of this energy is released through acoustic waves. This released fraction is often considered to be proportional to the total kinetic energy during the avalanche: $dE_{AE} \propto |v(t)|^2 dt$. Thus, if the AE sensor returns a voltage signal $V(t)$ proportional to the detected wave, we can naively interpret $dE_{AE} \propto |V(t)|^2 dt$. However, AE detection equipments typically have a limited bandwidth and might fail to capture the energy of high frequency events accurately. Additionally, the acoustic response might not be proportional to the original signal if the material damping is low and the signal resonates in delayed wave trains. As an alternative, the time integral ($E_{AE}$) of an AE event is sometimes considered proportional to the peak value of the kinetic energy: $E_{AE} \propto K \propto |v_{\max}|^2$. Both interpretations of the energy are compatible with two extreme limiting cases of a simple model for the modulation of the signal, as described in Ref. [S24]. We model the voltage signal as the convolution of the slip velocity $v(t)$ with a damped oscillation:

$$V(t) = G\int_{-\infty}^{t} v(t)e^{i\omega_0 t - \frac{t-t'}{\tau}}dt' \quad \text{(S9)}$$

where $\tau$ is the characteristic attenuation time of the signal and $\omega_0$ a resonant frequency. Let's consider a single event at time $t_i$. If the acoustic wave has an attenuation time $\tau$ longer than the typical avalanche duration $T$ the recorded signal will have a typical profile $|V(t)| \sim |v_{\max}(t)|\exp\left(\frac{t_i-t}{\tau}\right)$ and the recorded energy $E_{AE} \propto |v_{\max}|^2$. The duration of the recorded signal ($D_{AE}$) before dropping below the threshold level will be related linearly to $\tau$ and logarithmically to the voltage: $D_{AE} \propto \tau\log(V_{\max})$. In the other extreme case, when $\tau \ll T$, the attenuation is sharp, the voltage has a similar profile to the avalanche $|V(t)| \sim |v(t)|$, and duration $D_{AE} \approx T$, and the energy can be interpreted as $E_{AE} \propto \int |v(t-t_i)|^2 dt$. By using this model, we can establish the relation between the energy $E_{AE}$, the duration $D$ and the amplitude of the signal $A := \max(V(t))$ given a voltage threshold above noise levels needed to define the signal.

We consider the scaling relationships in Eqs. (S1–S3), from which the exponent relation $\frac{1}{\sigma\nu z} \equiv \frac{\gamma+1}{2}$ can be derived given the definition used in Eq. (4) of Ref. [S1]. Instead of working with signal profiles that are too noisy in this kind of experiments, we interpret the magnitudes of the recorded signals: $A_{AE}, E_{AE}, D_{AE}$, in terms of the MF theory and the corrected signal model to interpret the results. An approximate solution for the relation between the magnitudes of the recorded signals according to this signal model is presented in Ref. [S24] where some approximations were made in order to solve the problem analytically. In this work, we use an exact numerical solution for a parabolic avalanche shape in Eq. (S1) that is predicted by the MF model [S4]:

$$\tilde{v}(t/T) = 4\left(t/T-(t/T)^2\right). \quad \text{(S10)}$$

As a simplified alternative, the uniform avalanche shape ($\tilde{v}(t/T) = \Theta(t/T)(1-\Theta(t/T-1))$, being $\Theta(x)$ the Heaviside step-function) gives similar results, and minor variations are only perceptible for large events. The voltage thresholds imposed in Eq. (S9) are selected from Table I in Ref. [S1]. The experimental resolution and saturation limits ($\delta t = 1$ $\mu$s and $v(t) \leq 80$ dB) are taken into account to define the hitting time $t_{AE}$ and duration $D_{AE}$ in the numerical results of the signal model. As

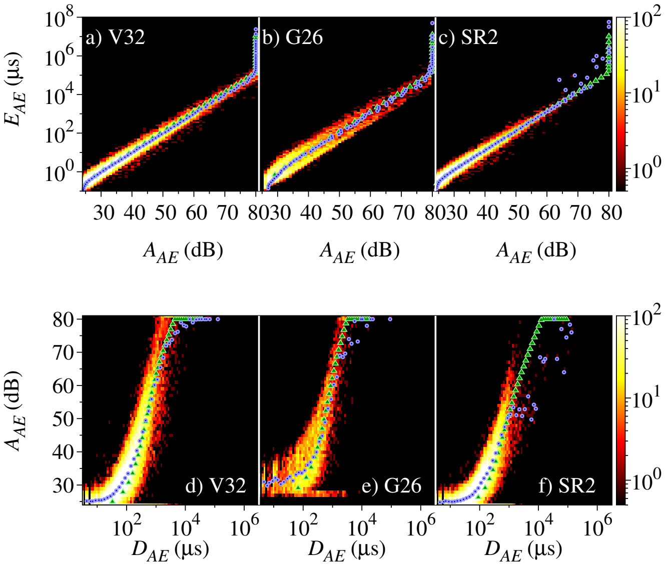


FIG. S1. (color online) Histograms of registered AE event-magnitudes $E(A)$ (top panels) and $A_{AE}(D_{AE})$(bottom panels). The average values $\langle A_{AE}\rangle(E_{AE})$ (top) and $\langle D_{AE}\rangle(A_{AE})$ (bottom) are represented in blue dots. The green triangles are obtained from the numerical solutions with the signal model given Eqs. (4) from Ref. [S1] and (S9) from the sum with $\tau = 100\mu$s, $\gamma = 3.0$ and $\log_{10} G = 13.4$ (V/m) for V32, $\tau = 125\mu$s, $\gamma = 3.4$ and $\log_{10} G = 14$ (V/m) for G26, $\tau = 125\mu$s, $\gamma = 3.2$ and $\log_{10} G = 13$ (V/m) for SR2.

reported in (Fig. 1) of Ref. [S1], the regime compatible with $E_{AE} \sim |v_{\max}|^2$ is observed for $T \ll \tau$ and the behavior transitions towards the regime $E_{AE} \sim \int |v(t)|^2 dt$ for $T \gg \tau$. For $D \gg \tau$, the naive relationship $\langle E|D\rangle \sim D^\gamma$ is consistent with the exponent values $\gamma \sim 3$. Fig. S1 is included to verify the signal model, by representing also the relations $E_{AE}, A_{AE}$ and $A_{AE}, D_{AE}$. The best parameters of the model are found by inspection. The exponent values $\gamma \approx 3$ (or $(\sigma\nu z)^{-1} \sim 2$) are compatible with the ones predicted by MF models [S2, S4].

### IV. Distribution of AE energies

The results presented in Fig. 3.d–f of Ref. [S1] are obtained form the AE catalogs divided in subcatalogs correlatives in time. In order to be statistically significant, the subcatalogs are selected with a time interval longer than a minimum $\delta t \propto f$ with respect to the next failure event and contain a number of at least $N$ =100 AE events (50 in the case of the more disperse catalog G26). The results are compared to the Ansatz given by Eq. (5) in Ref. [S1] giving an energy complementary cumulative

| | $E_m$ (aJ) | $n_{\min}$ | $E_c$ (aJ) | $\langle n\rangle$ | $\varepsilon$ |
|---|---|---|---|---|---|
| V32 | 1 | 100 | $10^6$ | 193(206) | 1.4 |
| G26 | 1 | 50 | $10^6$ | 86(103) | 1.4 |
| SR2 | 1 | 100 | $10^4$ | 97(141) | 1.6 |

TABLE SI. List of parameters used for the EVT analysis shown in Fig. S3 considering the validity of Eq. (S11): $E_c$ and $n_{\min}$ are the imposed lower cutoff and minimum number of events per subcatalog; $E_c$ is the broad approximation for the characteristic scale of the upper exponential cutoff to the distribution; $\langle n\rangle$ is the average number of events per subcatalog (standard deviation in brackets); $\varepsilon$ is the exponent assumed to be the most common in all subcatalogs.

distribution function (CCDF):

$$\mathrm{CCDF}(E; E_m, E_c, \varepsilon) = \frac{\Gamma\left(1-\varepsilon, \frac{E}{E_c}\right)}{\Gamma\left(1-\varepsilon, \frac{E_m}{E_c}\right)}, \qquad \text{(S11)}$$

with the fitted exponent $\varepsilon$, $E_m$= 1 aJ and $E_c = 10^6$ aJ ($10^4$ aJ for SR2), that work as a reasonable guide to the eye for most of the subcatalogs. The average energy ($\langle E_{AE}\rangle$) in the last subcatalogs right before failure is systematically above the Ansatz prediction, and could be related to an increase of $E_c$ as expected by critical failure. Here, we show the full experimental CCDF($E_{AE}$) for the subcatalogs to understand the variations in $\langle E_{AE}\rangle$ observed in Fig. 3 of Ref. [S1].

Fig. S2 shows the CCDF for different subcatalogs broken down into individual failure points. The CCDF predicted by the Ansatz for the estimated exponent ($\widehat{\varepsilon}_k$) within the energy interval 1–1000 aJ is shown as a solid curve in a lighter color. Apart from the last time intervals (black lines), the distributions do not exhibit a systematic variation of the exponent nor of the cutoff as function of the proximity to failure. In some limited cases the fitted values $\widehat{\varepsilon}_k$ do not agree with the numerical CCDF. The particular case represented as the green line in G26: k=4, is easily identified as a clear outlier with high $\widehat{\varepsilon}_k$ in Fig. 3.b of Ref. [S2]. The magnitude of the cutoff, related to $E_c$ still fluctuates up to three decades within such short time intervals (see V32: k=4 and k=5). The range of such fluctuations in the cutoff is compatible with the expectations of the extreme value theory (EVT). To verify that, Fig. S3 shows a logarithmic binning of the maximum energies ($E_{\max}$) found in all subcatalogs, excluding the last ones before failure (black lines in Fig. S2). The solid lines represent the expected numbers from EVT considering Eq. (S11) and the parameters shown in Table SI. As an exception, SR2 is compared to the solution with $\varepsilon = 1.6$ that seems to be the most common exponent in the subcatalogs shown in Fig. 3.c of Ref. [S1]. Since the number of elements in each subcatalog is not the same, an average is shown as a dark

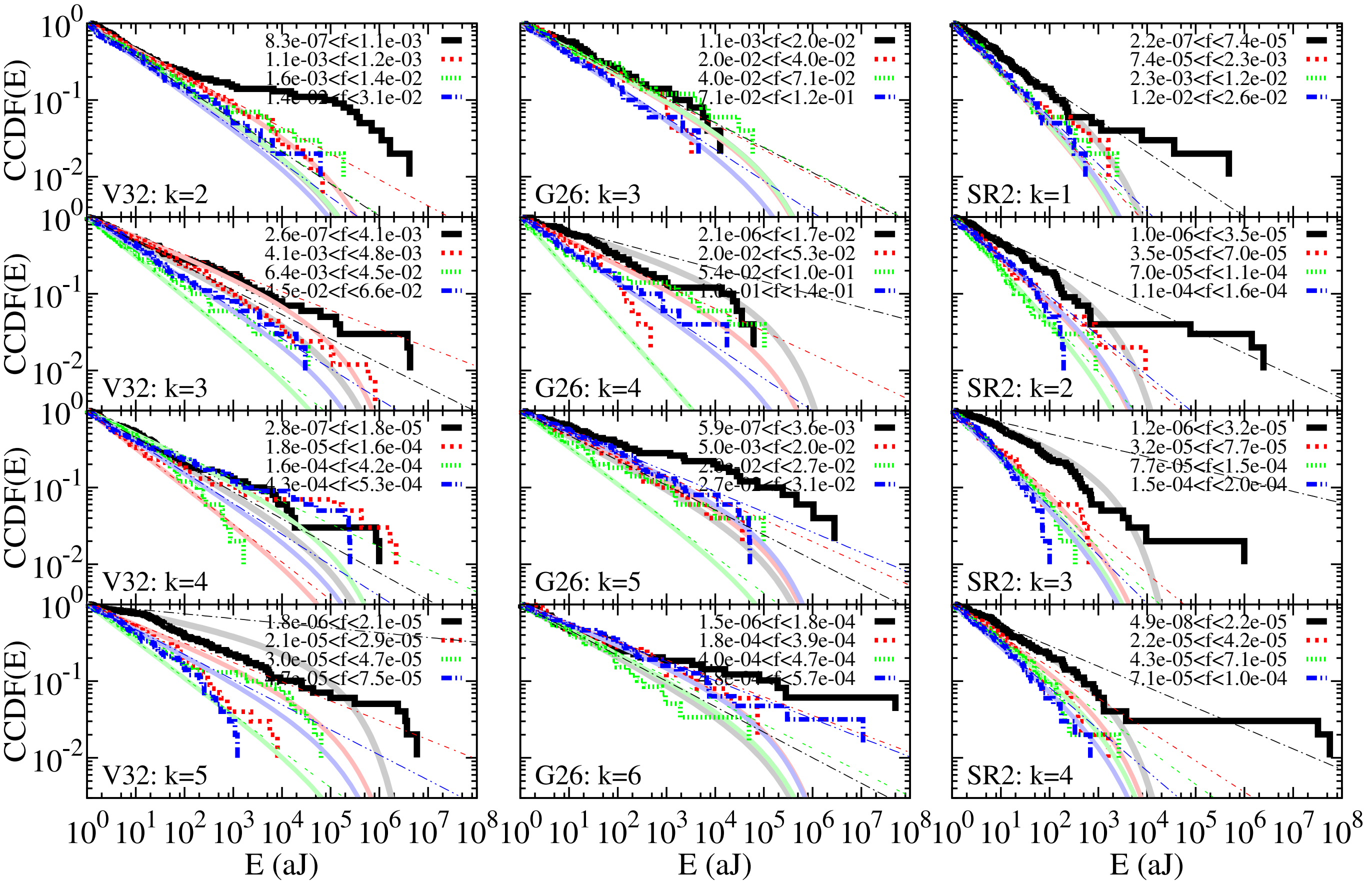


FIG. S2. (color online) Complementary cumulative distribution functions (CCDF) of AE-energies in the subcatalogs closer to the last four strain drops in each experiment, as the most relevant examples. Black lines represent the last interval containing the 100 (50 in G26) last AE-events before the strain drops. Red, green and blue correspond to the previous intervals in reverse order. The theoretical CCDF with estimated exponent $\widehat{\varepsilon}$ and equal $E_C$ are represented as lighter curves in the same colors . dashed lines. The power-law approximate solutions are given $\widehat{\varepsilon}$ are represented as thin dashed lines.

line. A limit of one standard deviation above and the imposed lower catalog size are shown as lighter lines in the same color. As a reference, grey lines represent the EVT solutions considering a pure power-law ($E_c \to \infty$). Although the details of the binned $N(E_{\max})$ are not entirely captured, it is obvious that the fluctuations on $E_{\max}$ observed as cutoffs in Fig. S2 are within the expectations of EVT in Fig. S3 and far below the expected by a pure power law. Thus, the observed variability in the intervals previous to failure can be explained as a mere statistical effect. On the contrary, the last intervals prior to failure (black lines in Fig. S2) stand out as clear outliers relative to the Ansatz given by Eq. S11. This disagreement can be identified as the superposition of a secondary population of large events, in some cases (see all $k$ values in SR2) several decades stronger than in previous intervals, and yielding, in most cases, a decrease of the estimated $\widehat{\varepsilon}_k$. In some cases, this population can extend to the previous intervals (see the red lines in V32: k=3 and k=4) while in others this population of large evens seems to be missing (see G26: k=3). While the variations in the avalanche statistics for these last intervals (black lines) are significant, we believe that the secondary population is already involved with brittle failure, localization phenomena or even some superposition of events which is beyond the predictions from critical failure. Fig. S2 corroborates that critical failure cannot predict the scaling of the CCDF of the AE energies observed in our experimental results.


* jordi.barourbea@ucalgary.ca
† eduard@fmc.ub.edu


[S1] Jordi Baró, Karin A. Dahmen, Jörn Davidsen, Antoni Planes, Pedro O. Castillo, Guillaume F. Nataf, Ekhard K. H. Salje, and Eduard Vives. Experimental evidence of accelerated seismic release without critical failure in acoustic emissions of compressed nanoporous materials. *(under review)*, 2018.

[S2] Jordi Baró and Jörn Davidsen. Universal avalanche statistics and triggering close to failure in a mean

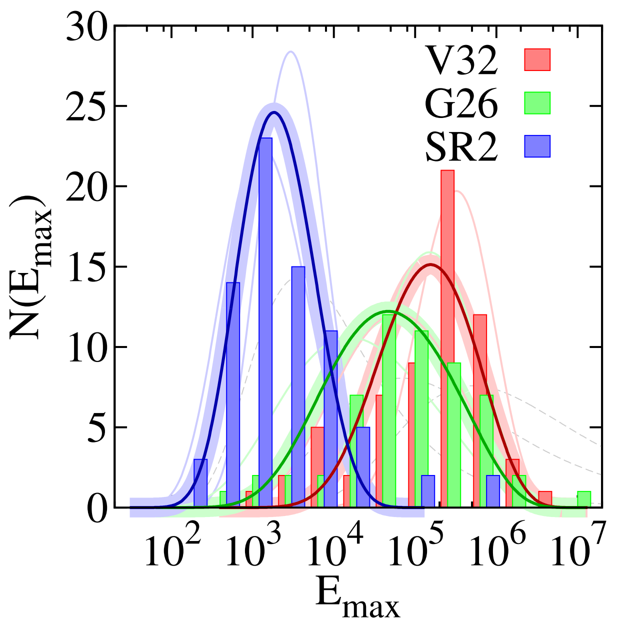


FIG. S3. (color online) Histograms: number of maximum energies ($E_{\max}$) of all subcatalogs in logarithmic bins. Dark lines: prediction of extreme value theory (EVT) considering Eq. (S11), the parameters in Table SI and a number of signals per subcatalog $n = \langle n \rangle$. The thin lines represent the extreme cases with a number of signals per subcatalog $n = n_{\min}$ and $n = \langle n \rangle + \mathrm{SD}(n)$. Grey lines indicate the extreme cases with $n = \langle n \rangle$ and $E_c \to \infty$.

field model of rheological fracture. *arXiv preprint arXiv:1801.01930 (accepted for publication in PRE)*, 2018.

[S3] Karin A Dahmen. Mean field theory of slip statistics. In *Avalanches in Functional Materials and Geophysics*, pages 19–30. Springer, 2017.

[S4] Karin A Dahmen, Yehuda Ben-Zion, and Jonathan T Uhl. Micromechanical model for deformation in solids with universal predictions for stress-strain curves and slip avalanches. *Physical Review Letters*, 102(17):175501, 2009.

[S5] Ekhard KH Salje and Karin A Dahmen. Crackling noise in disordered materials. *Annual Review of Condensed Matter Physics*, 5(1):233–254, 2014.

[S6] Yehuda Ben-Zion and James R Rice. Earthquake failure sequences along a cellular fault zone in a three-dimensional elastic solid containing asperity and nonasperity regions. *Journal of Geophysical Research: Solid Earth*, 98(B8):14109–14131, 1993.

[S7] Daniel S Fisher, Karin Dahmen, Sharad Ramanathan, and Yehuda Ben-Zion. Statistics of earthquakes in simple models of heterogeneous faults. *Physical Review Letters*, 78(25):4885, 1997.

[S8] R Burridge and Leon Knopoff. Model and theoretical seismicity. *Bulletin of the seismological society of america*, 57(3):341–371, 1967.

[S9] Zeev Olami, Hans Jacob S Feder, and Kim Christensen. Self-organized criticality in a continuous, nonconservative cellular automaton modeling earthquakes. *Physical Review Letters*, 68(8):1244, 1992.

[S10] Lucas Girard, Jérôme Weiss, and David Amitrano. Damage-cluster distributions and size effect on strength in compressive failure. *Physical Review Letters*, 108(22):225502, 2012.

[S11] Nir Friedman, Andrew T Jennings, Georgios Tsekenis, Ju-Young Kim, Molei Tao, Jonathan T Uhl, Julia R Greer, and Karin A Dahmen. Statistics of dislocation slip avalanches in nanosized single crystals show tuned critical behavior predicted by a simple mean field model. *Physical Review Letters*, 109(9):095507, 2012.

[S12] R Maaß, M Wraith, JT Uhl, JR Greer, and KA Dahmen. Slip statistics of dislocation avalanches under different loading modes. *Physical Review E*, 91(4):042403, 2015.

[S13] Yehuda Ben-Zion, Karin A Dahmen, and Jonathan T Uhl. A unifying phase diagram for the dynamics of sheared solids and granular materials. *Pure and Applied Geophysics*, 168(12):2221–2237, 2011.

[S14] Karin A Dahmen, Yehuda Ben-Zion, and Jonathan T Uhl. A simple analytic theory for the statistics of avalanches in sheared granular materials. *Nature Physics*, 7(7):554, 2011.

[S15] Jonathan T Uhl, Shivesh Pathak, Danijel Schorlemmer, Xin Liu, Ryan Swindeman, Braden AW Brinkman, Michael LeBlanc, Georgios Tsekenis, Nir Friedman, Robert Behringer, et al. Universal quake statistics: from compressed nanocrystals to earthquakes. *Scientific reports*, 5:16493, 2015.

[S16] Wendelin J Wright, Yun Liu, Xiaojun Gu, Katherine D Van Ness, Steven L Robare, Xin Liu, James Antonaglia, Michael LeBlanc, Jonathan T Uhl, Todd C Hufnagel, et al. Experimental evidence for both progressive and simultaneous shear during quasistatic compression of a bulk metallic glass. *Journal of Applied Physics*, 119(8):084908, 2016.

[S17] DV Denisov, KA Lörincz, JT Uhl, KA Dahmen, and P Schall. Universality of slip avalanches in flowing granular matter. *Nature communications*, 7:10641, 2016.

[S18] Dmitry V Denisov, Kinga A Lőrincz, Wendelin J Wright, Todd C Hufnagel, Aya Nawano, Xiaojun Gu, Jonathan T Uhl, Karin A Dahmen, and Peter Schall. Universal slip dynamics in metallic glasses and granular matter–linking frictional weakening with inertial effects. *Scientific Reports*, 7, 2017.

[S19] James Antonaglia, Xie Xie, Gregory Schwarz, Matthew Wraith, Junwei Qiao, Yong Zhang, Peter K Liaw, Jonathan T Uhl, and Karin A Dahmen. Tuned critical avalanche scaling in bulk metallic glasses. *Scientific Reports*, 4, 2014.

[S20] Michael LeBlanc, Aya Nawano, Wendelin J Wright, Xiaojun Gu, Jonathan T Uhl, and Karin A Dahmen. Avalanche statistics from data with low time resolution. *Physical Review E*, 94(5):052135, 2016.

[S21] Srutarshi Pradhan and Bikas K Chakrabarti. Precursors of catastrophe in the bak-tang-wiesenfeld, manna, and random-fiber-bundle models of failure. *Physical Review E*, 65(1):016113, 2001.

[S22] F Kun, F Raischel, RC Hidalgo, and HJ Herrmann. Extensions of fibre bundle models. In *Modelling Critical and Catastrophic Phenomena in Geoscience*, pages 57–92. Springer, 2006.

[S23] Raúl Cruz Hidalgo, Christian U Grosse, Ferenc Kun, Hans W Reinhardt, and Hans J Herrmann. Evolution of

percolating force chains in compressed granular media. *Physical Review Letters*, 89(20):205501, 2002.
[S24] Eduard Vives, Jordi Baró, and Antoni Planes. From labquakes in porous materials to earthquakes. In *Avalanches in Functional Materials and Geophysics*, pages 31–58. Springer, 2017.
